# Supplementary material for: CoATA: Effective Co-Augmentation of Topology and Attribute for Graph Neural Networks
Source: arXiv:2506.22299 source file (2025-06-27)
Supplement: Supplementary file 1 [file appendix.tex]

\clearpage
\appendix
\section{Appendix} \label{appendix：proof}
\subsection{Missing Proofs}

\begin{theorem}[Convergence of Higher-Order Attribute Propagation]\label{thom:convergence}
Let \(\mathbf{\tilde{A}}\) be a normalized adjacency matrix satisfying \(\|\mathbf{\tilde{A}}\| \le 1\) (e.g., in terms of the spectral norm or row-sum norm), and let the residual coefficient \(\beta \in (0,1]\). Define the iterative update
\[
\mathbf{X}^{(l)} = (1 - \beta)\,\mathbf{\tilde{A}}\,\mathbf{X}^{(l-1)} + \beta\,\mathbf{X},\quad \mathbf{X}^{(0)} = \mathbf{X}.
\]
Then the sequence \(\{\mathbf{X}^{(l)}\}\) converges to the unique fixed point
\[
\mathbf{X}^* = \beta\,\left(\mathbf{I} - (1-\beta)\,\mathbf{\tilde{A}}\right)^{-1}\mathbf{X}.
\]
\end{theorem}

\begin{proof}
Define the error term as \(\mathbf{E}^{(l)} = \mathbf{X}^{(l)} - \mathbf{X}^*\), where \(\mathbf{X}^*\) is the fixed point,considering the iterative update formula,we obtain:
\[
\begin{aligned}
\mathbf{E}^{(l)} &= (1 - \beta)\,\mathbf{\tilde{A}}\,\mathbf{E}^{(l-1)} \\
&= (1 - \beta)^2 \mathbf{\tilde{A}}^2 \mathbf{E}^{(l-2)} \\
&\quad \vdots \\
&= (1 - \beta)^l \mathbf{\tilde{A}}^l \mathbf{E}^{(0)}.
\end{aligned}
\]

Since \(\|\mathbf{\tilde{A}}\| \leq 1\) and \(0 < 1 - \beta < 1\), it follows that:
\[
\|\mathbf{E}^{(l)}\| \leq (1 - \beta)^l \|\mathbf{\tilde{A}}^l\| \|\mathbf{E}^{(0)}\| \leq (1 - \beta)^l \|\mathbf{E}^{(0)}\|.
\]
Taking the limit as \( l \to \infty \), we obtain \(\|\mathbf{E}^{(l)}\| \to 0\), Thus, \(\mathbf{X}^{(l)}\) converges to the fixed point \(\mathbf{X}^*\).

Next, we solve for \(\mathbf{X}^*\). Setting \(\mathbf{X}^{(l)} = \mathbf{X}^*\) in the iterative update formula, we obtain:
\[
\mathbf{X}^* = (1 - \beta)\,\mathbf{\tilde{A}}\,\mathbf{X}^* + \beta\,\mathbf{X}.
\]
Rearranging gives:
\[
\mathbf{X}^* - (1 - \beta)\,\mathbf{\tilde{A}}\,\mathbf{X}^* = \beta\,\mathbf{X},
\]
\[
(\mathbf{I} - (1 - \beta)\,\mathbf{\tilde{A}})\mathbf{X}^* = \beta\,\mathbf{X}.
\]
Since \(\|\mathbf{\tilde{A}}\| \leq 1\) and \(0 < 1 - \beta < 1\), the matrix \(\mathbf{I} - (1 - \beta)\,\mathbf{\tilde{A}}\) is invertible, and its inverse can be expressed as:
\[
\mathbf{X}^* = \beta \left(\mathbf{I} - (1 - \beta)\,\mathbf{\tilde{A}}\right)^{-1} \mathbf{X}.
\]
This completes the proof. \(\square\)
\end{proof}

\begin{theorem}[Prototype Alignment Guarantee]\label{thm:proto_align}
Minimizing the contrastive loss \(\mathcal{L}_{dpa}\) ensures that prototypes from the same class across channels are pulled closer (\(\cos(\mathbf{p}_j, \mathbf{p}_j') \to 1\)) while those from different classes remain separated (\(\cos(\mathbf{p}_j, \mathbf{p}_q')\) is bounded away from 1 for \(j \neq q\)).
\end{theorem}

\begin{proof}
For each class \(j\), we define the contrastive loss component as
\[
\ell_j = -\log \frac{\exp\left(\frac{\cos(\mathbf{p}_j,\mathbf{p}_j')}{\tau}\right)}{\sum_{q\neq j}\exp\left(\frac{\cos(\mathbf{p}_j,\mathbf{p}_q')}{\tau}\right)},
\]
and introduce the scaled similarity scores
\[
s_{jq} = \frac{\cos(\mathbf{p}_j,\mathbf{p}_q')}{\tau}.
\]
Thus, the loss can be rewritten as
\[
\ell_j = -s_{jj} + \log\left(\sum_{q\neq j}\exp(s_{jq})\right).
\]

Taking the gradient of \(\ell_j\) with respect to \(\mathbf{p}_j\) yields
\[
\nabla_{\mathbf{p}_j}\ell_j = -\frac{1}{\tau}\nabla_{\mathbf{p}_j}\cos(\mathbf{p}_j,\mathbf{p}_j') + \frac{1}{\tau}\sum_{q\neq j}\frac{\exp(s_{jq})}{\sum_{k\neq j}\exp(s_{jk})}\nabla_{\mathbf{p}_j}\cos(\mathbf{p}_j,\mathbf{p}_q').
\]
Noting via the chain rule that
\[
\nabla_{\mathbf{p}_j} s_{jq} = \frac{1}{\tau}\nabla_{\mathbf{p}_j}\cos(\mathbf{p}_j,\mathbf{p}_q'),
\]
we identify two key effects:

      \stitle{\textbf{(1) Positive Alignment:}} The term

    \[
    -\frac{1}{\tau}\nabla_{\mathbf{p}_j}\cos(\mathbf{p}_j,\mathbf{p}_j')
    \]
    directly increases \(\cos(\mathbf{p}_j,\mathbf{p}_j')\), thereby pulling the prototype \(\mathbf{p}_j\) closer to its corresponding prototype \(\mathbf{p}_j'\) from the other channel.
    
  \stitle{\textbf{(2) Negative Separation:}} The term
    \[
    \frac{1}{\tau}\sum_{q\neq j}\frac{\exp(s_{jq})}{\sum_{k\neq j}\exp(s_{jk})}\nabla_{\mathbf{p}_j}\cos(\mathbf{p}_j,\mathbf{p}_q')
    \]
    applies a repulsive force on the similarity between \(\mathbf{p}_j\) and prototypes \(\mathbf{p}_q'\) from different classes. The softmax weighting
    \(\frac{\exp(s_{jq})}{\sum_{k\neq j}\exp(s_{jk})}\) ensures that negatives with higher similarity are penalized more, thus reinforcing the separation.

At equilibrium, where \(\nabla_{\mathbf{p}_j}\ell_j = \mathbf{0}\), the positive alignment term must balance the weighted sum of the negative gradients:
\[
\nabla_{\mathbf{p}_j}\cos(\mathbf{p}_j,\mathbf{p}_j') = \sum_{q\neq j}\frac{\exp(s_{jq})}{\sum_{k\neq j}\exp(s_{jk})}\nabla_{\mathbf{p}_j}\cos(\mathbf{p}_j,\mathbf{p}_q').
\]
This balance can only occur if the similarity between \(\mathbf{p}_j\) and its positive pair \(\mathbf{p}_j'\) is maximized (i.e., \(\cos(\mathbf{p}_j,\mathbf{p}_j')\to 1\)) while the similarities with negative pairs remain strictly lower. In particular, there exists some \(\epsilon > 0\) such that for all \(q\neq j\):
\[
\cos(\mathbf{p}_j,\mathbf{p}_q') \le 1-\epsilon.
\]

In other words, the loss \(\ell_j\) is minimized when the positive similarity is the maximum element of the set:
\[
\mathcal{S}_j = \{\cos(\mathbf{p}_j,\mathbf{p}_q') : q=1,\dots,c\},
\]
with a gap of at least \(\delta > 0\) to the highest negative similarity:
\[
\cos(\mathbf{p}_j,\mathbf{p}_j') = \max \mathcal{S}_j \quad \text{and} \quad \max_{q\neq j}\cos(\mathbf{p}_j,\mathbf{p}_q') \le \cos(\mathbf{p}_j,\mathbf{p}_j') - \delta.
\]

Thus, minimizing the overall contrastive loss
\[
\mathcal{L}_{dpa} = \frac{1}{2c}\sum_{j=1}^c \ell_j
\]
via gradient descent drives \(\cos(\mathbf{p}_j,\mathbf{p}_j')\) toward 1, while ensuring that \(\cos(\mathbf{p}_j,\mathbf{p}_q')\) for \(q\neq j\) remains bounded away from 1. This completes the proof that prototypes from the same class across channels are pulled closer, whereas those from different classes are kept apart.
\end{proof}

\begin{theorem}[Lower Bound for Bipartite PPR]\label{thm:tight-ppr-bound}
Let \( G_b = (V \cup U, E_b) \) be a bipartite graph with node set \( V \), attribute set \( U \), and edge weights satisfying
$ w(a,v) \ge w_{\min}\ \text{for all } (a,v) \in E_b.$
Define
$
d_{\max}^V := \max_{v \in V} d(v),\ d_{\max}^U := \max_{a \in U} d(a).
$
For any target node \( v_j \) reachable from a source \( s \) via at least one length-\(2c\) path, the Personalized PageRank (PPR) score satisfies
\[
\pi(v_j) \ge \alpha (1-\alpha)^{2c} \cdot \left|\mathcal{P}_{2c}(s \leadsto v_j)\right| \cdot \left(\frac{w_{\min}^2}{d_{\max}^V d_{\max}^U}\right)^c.
\]
\end{theorem}

\begin{proof}
Let the random walk matrix for the bipartite graph \(G_b\) be defined as \(\mathbf{M} = \mathbf{D}^{-1}\mathbf{W}\), where \(\mathbf{W}\) is the weighted adjacency matrix and \(\mathbf{D}\) is the corresponding diagonal degree matrix.

In a bipartite graph, any valid path from a source \( s \in V \) to a target \( v_j \in V \) must have even length, alternating between nodes in \( V \) and attributes in \( U \). Specifically, consider a length-\(2c\) path
\[
p: \quad v_0 \to a_1 \to v_1 \to a_2 \to v_2 \to \cdots \to a_c \to v_c,
\]
with \( v_0 = s \) and \( v_c = v_j \). For a single two-hop transition from \( v_{i-1} \) to \( v_i \) via \( a_i \), the transition probability is
$\frac{w(v_{i-1}, a_i)}{d(v_{i-1})} \cdot \frac{w(a_i, v_i)}{d(a_i)}.$
Our preprocessing guarantees that
$w(v_{i-1}, a_i) \ge w_{\min},w(a_i, v_i) \ge w_{\min},$
and since $d(v_{i-1}) \le d_{\max}^V,d(a_i) \le d_{\max}^U,$
we have
\[
\frac{w(v_{i-1}, a_i)}{d(v_{i-1})} \cdot \frac{w(a_i, v_i)}{d(a_i)}
\ge \frac{w_{\min}}{d_{\max}^V} \cdot \frac{w_{\min}}{d_{\max}^U} = \frac{w_{\min}^2}{d_{\max}^V d_{\max}^U}.
\]
Taking the product over all \( c \) two-hop transitions along the path \( p \) yields
\[
\prod_{i=1}^{c} \left(\frac{w(v_{i-1}, a_i)}{d(v_{i-1})} \cdot \frac{w(a_i, v_i)}{d(a_i)}\right)
\ge \left(\frac{w_{\min}^2}{d_{\max}^V d_{\max}^U}\right)^c.
\]
Summing over all length-\(2c\) paths from \( s \) to \( v_j \), denoted by \(\mathcal{P}_{2c}(s \leadsto v_j)\), we obtain
\[
(\mathbf{M}^{2c})_{s,v_j} \ge \left|\mathcal{P}_{2c}(s \leadsto v_j)\right| \cdot \left(\frac{w_{\min}^2}{d_{\max}^V d_{\max}^U}\right)^c.
\]
Finally, by the definition of the Personalized PageRank (PPR) vector, and noting that in a bipartite graph only even-length paths contribute, we have
\[
\begin{aligned}
\pi(v_j) &= \alpha \sum_{r=0}^{\infty} (1-\alpha)^r (\mathbf{M}^r)_{s,v_j} \\
&\ge \alpha (1-\alpha)^{2c} (\mathbf{M}^{2c})_{s,v_j} \\
&\ge \alpha (1-\alpha)^{2c} \cdot \left|\mathcal{P}_{2c}(s \leadsto v_j)\right| \cdot \left(\frac{w_{\min}^2}{d_{\max}^V d_{\max}^U}\right)^c.
\end{aligned}
\]
\end{proof}

\subsection{Missing Algorithm}
The training process of CoATA is summarized in Algorithm~\ref{alg:CoATA}, which is self-explanatory and we omit the detailed explanation for it.

\subsection{Additional Experiments}
\begin{algorithm}[t]
\caption{\textit{The training algorithm of CoATA}}
\label{alg:CoATA}
\footnotesize
\begin{flushleft}
\textbf{Input:} Feature matrix $\mathbf{X}$; Adjacency matrix $\mathbf{\tilde{A}}$; Training label matrix $\mathbf{Y}_L$. \\
\textbf{Parameters:} Number of epochs $E$; Propagation steps $h$; Residual coefficient $\beta$; Number of neighbors $k$; Temperature $\tau$; Trade-off coefficients $\lambda_1, \lambda_2, \lambda_3$.\\
\hspace{0.35cm} \textcolor{blue}{\texttt{/* Pre-processing */}}\vspace{-0.1cm} 
\end{flushleft}
\begin{algorithmic}[1]
    \STATE Calculate ${\mathbf{H}} \leftarrow \text{Higher-order propagation}(\mathbf{X}, \mathbf{\tilde{A}}; h, \beta)$ \hfill \textit{// TEA}
    \STATE Construct node-attribute bipartite graph $\mathbf{G_b} \leftarrow \text{Bipartite-Graph}(\mathbf{H})$ 
    \STATE Calculate $\mathbf{\hat{\pi}} \leftarrow \text{Push-PPR}(\mathbf{G_b}, \alpha, r_{\max})$ 
    \STATE Calculate $ \mathbf{\tilde{A}^{(c)} } \leftarrow \text{KNN}(\mathbf{\tilde{A}}, \mathbf{\hat{\pi}}, K)$\hfill \textit{// AIT} 
    \STATE Calculate $\mathbf{\tilde{A}^{(c)} }\leftarrow \text{EdgeModification}(\mathbf{\tilde{A}}, \mathbf{\hat{\pi}}, k_{\mathrm{add}}, k_{\mathrm{del}})$

\textcolor{blue}{\texttt{/* Model Training */}}
\FOR {$e = 1, 2, \dots, E$}
    \STATE Calculate $\hat{\mathbf{Y}} \leftarrow \text{GNN}(\mathbf{\tilde{A}}, \mathbf{X})$ \hfill \textit{// Original channel}
    \STATE Calculate $\hat{\mathbf{Y}}' \leftarrow \text{GNN}(\mathbf{\tilde{A}^{(c)} }, \mathbf{X})$ \hfill \textit{// Augmented channel}
    
    \STATE Calculate $\mathcal{L}_{ce}$ from $\hat{\mathbf{Y}}, \mathbf{Y}_L$ \hfill \textit{// Cross-entropy}
    \STATE Calculate $\mathcal{L}_{ce}'$ from $\hat{\mathbf{Y}}', \mathbf{Y}_L$ 
    
    \STATE Calculate $\mathcal{L}_{co}$ from $\hat{\mathbf{Y}}'_s$ and $\mathbf{Y}^{\mathrm{agg}}$ \hfill \textit{// Consistency loss} 
    \STATE Calculate $\mathbf{Z}, \mathbf{Z'}$ from the linear projection layer 
    
    \STATE Calculate $\mathbf{p}_1, \dots, \mathbf{p}_c \leftarrow \text{Allocate-Prototypes}(\mathbf{Z}, \mathbf{Y}_L)$ \hfill \textit{// Allocate prototypes}
    \STATE Calculate $\mathbf{p}_1', \dots, \mathbf{p}_c' \leftarrow \text{Allocate-Prototypes}(\mathbf{Z'}, \mathbf{Y}_L)$  
    \STATE Calculate $\mathcal{L}_{dpa}$ from $\mathbf{p}_1, \dots, \mathbf{p}_c, \mathbf{p}_1', \dots, \mathbf{p}_c'$ and $\tau$ \hfill \textit{// DPA}
    \STATE Calculate total loss $\mathcal{L}$ from $\mathcal{L}_{ce}, \mathcal{L}_{ce}', \mathcal{L}_{co}, \mathcal{L}_{dpa}$ and $\lambda_1, \lambda_2, \lambda_3$
    
    \STATE Update model parameters via gradient descent
\ENDFOR
\end{algorithmic}
\end{algorithm}

\stitle{Dataset details.}
We evaluate our solutions on seven standard graph benchmarks, categorized into citation networks, co-authorship networks, and heterophilic graphs. These datasets provide diverse graph structures, enabling a comprehensive evaluation of graph-based learning models. Below are the details of each category:

\begin{itemize}[leftmargin=1.5em]
    \item \textbf{Cora, CiteSeer, and PubMed} are three citation networks, where each node represents a paper and each edge denotes a citation relationship. The attributes are the bag-of-words representations of paper content.
    \item \textbf{Coauthor-CS and Coauthor-Physics} are two co-authorship networks derived from the Microsoft Academic Graph. In these graph datasets, each node represents an author, and each edge is a co-authorship relationship between two authors. The attributes are the bag-of-words embeddings of keywords from authors' papers.
    \item \textbf{Squirrel and Chameleon} are web page networks with nodes representing web pages and edges as hyperlinks. These datasets exhibit strong heterophily, where connected nodes often belong to different categories. The attributes include structural and textual features of web pages. We used the filtered versions of these datasets, after removing duplicate nodes that shared the same regression target and neighborhood, to avoid data leakage in model evaluation ~\cite{heterograph}.
\end{itemize}

\begin{figure}[t]
  \centering
  \includegraphics[width=0.9\linewidth]{fig/ablation_separated_fixed.pdf} % 图的路径
  \vspace{-2mm}
  \caption{Accuracy w.r.t. \(\beta\)} % 
  \label{fig:tsne_coata} % 
\end{figure}

\stitle{Supplementary test.}
In addition to the main results presented in the body of the paper, we further supplement our findings with additional ablation experiments and parameter analyses. Specifically, we provide a comparison between \textit{CoATA} with and without the DPA mechanism on two representative homophilic and heterophilic graphs, extending the analysis to a wider range of values for the residual coefficient \(\beta\), as defined in Eq.4. Fig.~\ref{fig:tsne_coata} illustrates these results, showing how \textit{CoATA} consistently outperforms the variant without DPA across different structural settings. Even for \(\beta > 0.6\), where attribute propagation reverts towards the original features and causes a decline in overall accuracy, the performance degradation of \textit{CoATA} remains relatively mild, thanks to the prototype-level alignment introduced by DPA. This helps mitigate the sharp accuracy drop observed when DPA is absent. These supplementary results further reinforce the robustness of \textit{CoATA} under varying conditions.
